# Supplementary material for: The enumeration of inversion sequences avoiding the patterns 201 and 210
Source: arXiv:2310.19632 ancillary file (2024-04-25)
Supplement: Supplementary file 1 [file invs-av-201-210-public-worksheet-pdf.pdf]

$$\begin{aligned}
&> \\
&> \text{restart} \\
&> \\
&> \\
&> \text{Phi} := f \rightarrow \frac{(f - \text{subs}(u = 1, f))}{u - 1} \\
&\quad \Phi := f \mapsto \frac{f - \text{subs}(u = 1, f)}{u - 1} \tag{1}
\end{aligned}$$

$$\begin{aligned}
&> \\
&> \\
&> a, b, c, h := A(x, u), B(x, u), C(x, u), H(x, u) \\
&\quad a, b, c, h := A(x, u), B(x, u), C(x, u), H(x, u) \tag{2}
\end{aligned}$$

$$\begin{aligned}
&> \# \text{ doing Phi[Phi[A + B]] symbolically gives 0 over 0 so we make a helper equation for H(x, u)} \\
&> \\
&> eq1 := a = 1 + x \cdot u \cdot (a + \text{Phi}(a))
\end{aligned}$$

$$eq1 := A(x, u) = 1 + xu \left( A(x, u) + \frac{A(x, u) - A(x, 1)}{u - 1} \right) \tag{3}$$

$$\begin{aligned}
&> eq2 := b = x \cdot u \cdot (2 \cdot b + \text{Phi}(b) + c) \\
&\quad eq2 := B(x, u) = xu \left( 2B(x, u) + \frac{B(x, u) - B(x, 1)}{u - 1} + C(x, u) \right) \tag{4}
\end{aligned}$$

$$\begin{aligned}
&> eq3 := c = x \cdot u \cdot (\text{Phi}(u \cdot h) + \text{Phi}(c) + c) \\
&\quad eq3 := C(x, u) = xu \left( \frac{uH(x, u) - H(x, 1)}{u - 1} + \frac{C(x, u) - C(x, 1)}{u - 1} + C(x, u) \right) \tag{5}
\end{aligned}$$

$$\begin{aligned}
&> eq4 := h = \text{Phi}(a + b) \\
&\quad eq4 := H(x, u) = \frac{A(x, u) + B(x, u) - A(x, 1) - B(x, 1)}{u - 1} \tag{6}
\end{aligned}$$

$$\begin{aligned}
&> \\
&> \\
&> eqs := [eq1, eq2, eq3, eq4] \\
&\quad eqs := \left[ A(x, u) = 1 + xu \left( A(x, u) + \frac{A(x, u) - A(x, 1)}{u - 1} \right), \right. \\
&\quad \quad B(x, u) = xu \left( 2B(x, u) + \frac{B(x, u) - B(x, 1)}{u - 1} + C(x, u) \right), \\
&\quad \quad C(x, u) = xu \left( \frac{uH(x, u) - H(x, 1)}{u - 1} \right. \\
&\quad \quad \quad \left. + \frac{C(x, u) - C(x, 1)}{u - 1} + C(x, u) \right), \\
&\quad \quad \left. H(x, u) = \frac{A(x, u) + B(x, u) - A(x, 1) - B(x, 1)}{u - 1} \right] \tag{7}
\end{aligned}$$

```
>
> eqs := map(eq → denom(rhs(eq)) · lhs(eq) - numer(rhs(eq)), eqs)
```

$$\begin{aligned} eqs := & [(u-1)A(x,u) - A(x,u)u^2x + A(x,1)ux \\ & - u+1, (u-1)B(x,u) - xu(2B(x,u)u + C(x,u)u \\ & - B(x,u) - B(x,1) - C(x,u)), (u-1)C(x,u) \\ & - xu(C(x,u)u + uH(x,u) - H(x,1) - C(x,1)), (u-1)H(x,u) \\ & - A(x,u) - B(x,u) + A(x,1) + B(x,1)] \end{aligned} \quad (8)$$

```
> eqs := {op(eqs)}:
>
>
>
>
> eqs := subs({A(x,u) = Axu, A(x,1) = Ax1, B(x,u) = Bxu, B(x,1) = Bx1, C(x,u) =
Cxu, C(x,1) = Cx1, H(x,u) = Hxu, H(x,1) = Hx1}, eqs);
```

$$\begin{aligned} eqs := & \{(u-1)Bxu \\ & - xu(2Bxuu + Cxuu - Bx1 - Bxu - Cxu), (u-1)Cxu \\ & - xu(Cxuu + uHxu - Cx1 - Hx1), (u-1)Axu - Axu u^2x \\ & + Ax1ux - u+1, (u-1)Hxu - Axu - Bxu + Ax1 + Bx1\} \end{aligned} \quad (9)$$

```
>
>
>
>
> with(PolynomialIdeals):
> PI := PolynomialIdeal(eqs, parameters = {x,u}):
> HilbertDimension(PI)
```

$$4 \quad (10)$$

```
> collect(Generators(EliminationIdeal(PI, {Axu, Ax1}))[1], Axu, factor)
```

$$Ax1ux + (-u^2x + u - 1)Axu - u + 1 \quad (11)$$

```
> resultant(%, coeff(%, Axu, 1), u)
```

$$x^2 (Ax1^2x - Ax1 + 1) \quad (12)$$

```
> new_eq1 := %/x^2
```

$$new\_eq1 := Ax1^2x - Ax1 + 1 \quad (13)$$

```
> eqs := eqs union {new_eq1}
```

$$\begin{aligned}
eqs := \{ & (u-1) Bxu \\
& - xu (2Bxuu + Cxuu - Bx1 - Bxu - Cxu), (u-1) Cxu \\
& - xu (Cxuu + uHxu - Cx1 - Hx1), (u-1) Axu - Axu u^2 x + Ax1 ux \\
& - u + 1, (u-1) Hxu - Axu - Bxu + Ax1 + Bx1, Ax1^2 x - Ax1 + 1 \}
\end{aligned} \tag{14}$$

```

>
>
> PI := PolynomialIdeal(eqs, parameters = {x, u}):
> HilbertDimension(PI)

```

$$3 \tag{15}$$

```

>
>
>
>
> big_eq := collect(Generators(EliminationIdeal(PI, {Cxu, Bx1, Cx1, Hx1}))[1], Cxu, factor)

```

$$\begin{aligned}
big\_eq := & (u-1)^2 (u^2x - u + 1) (2u^2x - u + 1)^2 (xu - 1)^2 Cxu^2 \\
& - u(u-1) (2u^2x - u + 1) (xu - 1) (4Bx1 u^4x^3 + 4Cx1 u^4x^3 + 4Hx1 u^4x^3 \\
& - 2Cx1 u^3x^3 - 2Hx1 u^3x^3 - 6Bx1 u^3x^2 - 6Cx1 u^3x^2 - 6Hx1 u^3x^2 + 2u^4x^2 \\
& + 4Bx1 u^2x^2 + 8Cx1 u^2x^2 + 8Hx1 u^2x^2 + 3x^2u^3 + 2Bx1 u^2x + 2Cx1 u^2x \\
& - 2Cx1 u x^2 + 2Hx1 u^2x - 2Hx1 u x^2 - 3u^3x - 2u^2x^2 - 2Bx1 ux - 4Cx1 xu \\
& - 4Hx1 xu + 2xCx1 + 2xHx1 + u^2 + 2xu - u) Cxu + u^2x (4Bx1^2 u^6x^4 \\
& + 8Bx1 Cx1 u^6x^4 + 8Bx1 Hx1 u^6x^4 + 4Cx1^2 u^6x^4 + 8Cx1 Hx1 u^6x^4 + 4Hx1^2 u^6x^4 \\
& - 4Bx1 Cx1 u^5x^4 - 4Bx1 Hx1 u^5x^4 - 4Cx1^2 u^5x^4 - 8Cx1 Hx1 u^5x^4 - 4Hx1^2 u^5x^4 \\
& - 8Bx1^2 u^5x^3 - 16Bx1 Cx1 u^5x^3 - 16Bx1 Hx1 u^5x^3 + 4Bx1 u^6x^3 - 8Cx1^2 u^5x^3 \\
& + Cx1^2 u^4x^4 - 16Cx1 Hx1 u^5x^3 + 2Cx1 Hx1 u^4x^4 + 4Cx1 u^6x^3 - 8Hx1^2 u^5x^3 \\
& + Hx1^2 u^4x^4 + 4Hx1 u^6x^3 + 4Bx1^2 u^4x^3 + 18Bx1 Cx1 u^4x^3 + 18Bx1 Hx1 u^4x^3 \\
& + 6Bx1 u^5x^3 + 14Cx1^2 u^4x^3 + 28Cx1 Hx1 u^4x^3 + 4Cx1 u^5x^3 + 14Hx1^2 u^4x^3 \\
& + 4Hx1 u^5x^3 + 4u^6x^3 + 5Bx1^2 u^4x^2 + 10Bx1 Cx1 u^4x^2 - 4Bx1 Cx1 u^3x^3 \\
& + 10Bx1 Hx1 u^4x^2 - 4Bx1 Hx1 u^3x^3 - 8Bx1 u^5x^2 - 4Bx1 u^4x^3 + 5Cx1^2 u^4x^2 \\
& - 7Cx1^2 u^3x^3 + 10Cx1 Hx1 u^4x^2 - 14Cx1 Hx1 u^3x^3 - 8Cx1 u^5x^2 - 7Cx1 u^4x^3 \\
& + 5Hx1^2 u^4x^2 - 7Hx1^2 u^3x^3 - 8Hx1 u^5x^2 - 7Hx1 u^4x^3 - 4u^5x^3 - 4Bx1^2 u^3x^2 \\
& - 16Bx1 Cx1 u^3x^2 - 16Bx1 Hx1 u^3x^2 - 3Bx1 u^4x^2 - 12Cx1^2 u^3x^2 + Cx1^2 u^2x^3 \\
& - 24Cx1 Hx1 u^3x^2 + 2Cx1 Hx1 u^2x^3 + 2Cx1 u^4x^2 + 2Cx1 u^3x^3 - 12Hx1^2 u^3x^2 \\
& + Hx1^2 u^2x^3 + 2Hx1 u^4x^2 + 2Hx1 u^3x^3 - 4u^5x^2 + u^4x^3 - Bx1^2 u^3x \\
& - 2Bx1 Cx1 u^3x + 6Bx1 Cx1 u^2x^2 - 2Bx1 Hx1 u^3x + 6Bx1 Hx1 u^2x^2 + 5Bx1 u^4x \\
& + 6Bx1 u^3x^2 - Cx1^2 u^3x + 9Cx1^2 u^2x^2 - 2Cx1 Hx1 u^3x + 18Cx1 Hx1 u^2x^2 \\
& + 5Cx1 u^4x + 9Cx1 u^3x^2 - Hx1^2 u^3x + 9Hx1^2 u^2x^2 + 5Hx1 u^4x + 9Hx1 u^3x^2 \\
& + 6u^4x^2 + Bx1^2 u^2x + 4Bx1 Cx1 u^2x + 4Bx1 Hx1 u^2x - 2Bx1 u^3x + 3Cx1^2 u^2x \\
& - 2Cx1^2 u x^2 + 6Cx1 Hx1 u^2x - 4Cx1 Hx1 u x^2 - 6Cx1 u^3x - 4Cx1 u^2x^2 \\
& + 3Hx1^2 u^2x - 2Hx1^2 u x^2 - 6Hx1 u^3x - 4Hx1 u^2x^2 + u^4x - 2x^2u^3 - 2Bx1 Cx1 ux \\
& - 2Bx1 Hx1 ux - Bx1 u^3 - 2Bx1 u^2x - 3Cx1^2 ux - 6Cx1 Hx1 ux - Cx1 u^3 \\
& - Cx1 u^2x - 3Hx1^2 ux - Hx1 u^3 - Hx1 u^2x - 2u^3x + Bx1 u^2 + Cx1^2 x + 2Cx1 Hx1 x \\
& + 2Cx1 u^2 + 2Cx1 xu + Hx1^2 x + 2Hx1 u^2 + 2Hx1 xu + u^2x - Cx1 u - Hx1 u)
\end{aligned}
\tag{16}$$

$$\begin{aligned}
> \\
> new\_eq2 := & \frac{factor(resultant(big\_eq, 2u^2x - u + 1, u))}{16 \cdot x^{10}}
\end{aligned}$$

$$\begin{aligned}
new\_eq2 := & Cx1^4x^4 + 4Cx1^3Hx1x^4 \\
& + 6Cx1^2Hx1^2x^4 + 4Cx1Hx1^3x^4 + Hx1^4x^4 \\
& + 4Bx1^2Cx1^2x^3 + 8Bx1^2Cx1Hx1x^3 \\
& + 4Bx1^2Hx1^2x^3 + 2Bx1Cx1^3x^3 \\
& + 6Bx1Cx1^2Hx1x^3 + 6Bx1Cx1Hx1^2x^3 \\
& + 2Bx1Hx1^3x^3 + 4Bx1^4x^2 + 4Bx1^3Cx1x^2 \\
& + 4Bx1^3Hx1x^2 + Bx1^2Cx1^2x^2 \\
& + 2Bx1^2Cx1Hx1x^2 + Bx1^2Hx1^2x^2 \\
& - 8Bx1Cx1^2x^3 - 16Bx1Cx1Hx1x^3 \\
& - 8Bx1Hx1^2x^3 - 4Cx1^3x^3 - 12Cx1^2Hx1x^3 \\
& - 12Cx1Hx1^2x^3 - 4Hx1^3x^3 - 16Bx1^3x^2 \\
& - 16Bx1^2Cx1x^2 - 16Bx1^2Hx1x^2 - Bx1Cx1^2x^2 \\
& - 2Bx1Cx1Hx1x^2 - Bx1Hx1^2x^2 + Cx1^3x^2 \\
& + 3Cx1^2Hx1x^2 + 6Cx1^2x^3 + 3Cx1Hx1^2x^2 \\
& + 12Cx1Hx1x^3 + Hx1^3x^2 + 6Hx1^2x^3 + 6Bx1^3x \\
& + 5Bx1^2Cx1x + 5Bx1^2Hx1x + 20Bx1^2x^2 \\
& + Bx1Cx1^2x + 2Bx1Cx1Hx1x + 6Bx1Cx1x^2 \\
& + Bx1Hx1^2x + 6Bx1Hx1x^2 - 5Cx1^2x^2 \\
& - 10Cx1Hx1x^2 - 5Hx1^2x^2 - 11x Bx1^2 \\
& - 5xBx1Cx1 - 5xBx1Hx1 - 8x^2Bx1 \\
& + Cx1^2x + 2Cx1Hx1x + 4x^2Cx1 + Hx1^2x \\
& + 4x^2Hx1 + 2Bx1^2 + Bx1Cx1 + Bx1Hx1 \\
& + 7xBx1 - xCx1 - xHx1 + x^2 - Bx1
\end{aligned} \tag{17}$$

```

>
>
>
>
> eqs := eqs union {new_eq2}:
>
>
> PI := PolynomialIdeal(eqs, parameters = {x, u}):
> HilbertDimension(PI)

```

2 (18)

```

>
> # the elimination below takes several minutes
> big_eq2 := Generators(EliminationIdeal(PI, {Cx1, Cru, Hx1}))[1]:
>
>
> # there are two non - trivial factors and we need to determine which is correct

```

$$> two\_poss := \frac{factor(subs(u = 1, big\_eq2))}{x^6}$$

$$\begin{aligned}
two\_poss := & (16Cx1^4x^{10} + 64Cx1^3Hx1x^{10} + 96Cx1^2Hx1^2x^{10} + 64Cx1Hx1^3x^{10} \\
& + 16Hx1^4x^{10} - 32Cx1^4x^9 - 128Cx1^3Hx1x^9 - 192Cx1^2Hx1^2x^9 - 128Cx1Hx1^3x^9 \\
& - 32Hx1^4x^9 + 32Cx1^4x^8 + 128Cx1^3Hx1x^8 + 192Cx1^2Hx1^2x^8 + 128Cx1Hx1^3x^8 \\
& + 32Hx1^4x^8 - 16Cx1^4x^7 - 64Cx1^3Hx1x^7 + 48Cx1^3x^8 - 96Cx1^2Hx1^2x^7 \\
& + 144Cx1^2Hx1x^8 + 96Cx1^2x^9 - 64Cx1Hx1^3x^7 + 144Cx1Hx1^2x^8 \\
& + 192Cx1Hx1x^9 - 16Hx1^4x^7 + 48Hx1^3x^8 + 96Hx1^2x^9 + 4Cx1^4x^6 \\
& + 16Cx1^3Hx1x^6 - 64Cx1^3x^7 + 24Cx1^2Hx1^2x^6 - 192Cx1^2Hx1x^7 - 176Cx1^2x^8 \\
& + 16Cx1Hx1^3x^6 - 192Cx1Hx1^2x^7 - 352Cx1Hx1x^8 + 4Hx1^4x^6 - 64Hx1^3x^7 \\
& - 176Hx1^2x^8 + 40Cx1^3x^6 + 120Cx1^2Hx1x^6 + 272Cx1^2x^7 + 120Cx1Hx1^2x^6 \\
& + 544Cx1Hx1x^7 + 256Cx1x^8 + 40Hx1^3x^6 + 272Hx1^2x^7 + 256Hx1x^8 \\
& - 8Cx1^3x^5 - 24Cx1^2Hx1x^5 - 260Cx1^2x^6 - 24Cx1Hx1^2x^5 - 520Cx1Hx1x^6 \\
& - 336Cx1x^7 - 8Hx1^3x^5 - 260Hx1^2x^6 - 336Hx1x^7 + 16x^8 + 160Cx1^2x^5 \\
& + 320Cx1Hx1x^5 + 112Cx1x^6 + 160Hx1^2x^5 + 112Hx1x^6 + 192x^7 - 59Cx1^2x^4 \\
& - 118Cx1Hx1x^4 + 100Cx1x^5 - 59Hx1^2x^4 + 100Hx1x^5 - 256x^6 + 12Cx1^2x^3 \\
& + 24Cx1Hx1x^3 - 120Cx1x^4 + 12Hx1^2x^3 - 120Hx1x^4 - 124x^5 - Cx1^2x^2 \\
& - 2Cx1Hx1x^2 + 55Cx1x^3 - Hx1^2x^2 + 55Hx1x^3 + 448x^4 - 12Cx1x^2 - 12Hx1x^2 \\
& - 365x^3 + Cx1x + Hx1x + 142x^2 - 27x + 2) (4Cx1^4x^6 + 16Cx1^3Hx1x^6 \\
& + 24Cx1^2Hx1^2x^6 + 16Cx1Hx1^3x^6 + 4Hx1^4x^6 - 8Cx1^4x^5 - 32Cx1^3Hx1x^5 \\
& - 48Cx1^2Hx1^2x^5 - 32Cx1Hx1^3x^5 - 8Hx1^4x^5 + 8Cx1^4x^4 + 32Cx1^3Hx1x^4 \\
& + 48Cx1^2Hx1^2x^4 + 32Cx1Hx1^3x^4 + 8Hx1^4x^4 - 4Cx1^4x^3 - 16Cx1^3Hx1x^3 \\
& + 12Cx1^3x^4 - 24Cx1^2Hx1^2x^3 + 36Cx1^2Hx1x^4 + 24Cx1^2x^5 - 16Cx1Hx1^3x^3 \\
& + 36Cx1Hx1^2x^4 + 48Cx1Hx1x^5 - 4Hx1^4x^3 + 12Hx1^3x^4 + 24Hx1^2x^5 + Cx1^4x^2 \\
& + 4Cx1^3Hx1x^2 - 16Cx1^3x^3 + 6Cx1^2Hx1^2x^2 - 48Cx1^2Hx1x^3 - 36Cx1^2x^4 \\
& + 4Cx1Hx1^3x^2 - 48Cx1Hx1^2x^3 - 72Cx1Hx1x^4 + Hx1^4x^2 - 16Hx1^3x^3 \\
& - 36Hx1^2x^4 + 10Cx1^3x^2 + 30Cx1^2Hx1x^2 + 26Cx1^2x^3 + 30Cx1Hx1^2x^2 \\
& + 52Cx1Hx1x^3 + 10Hx1^3x^2 + 26Hx1^2x^3 - 2Cx1^3x - 6Cx1^2Hx1x + Cx1^2x^2 \\
& - 6Cx1Hx1^2x + 2Cx1Hx1x^2 + 36Cx1x^3 - 2Hx1^3x + Hx1^2x^2 + 36Hx1x^3 \\
& + 4x^4 - 5Cx1^2x - 10Cx1Hx1x - 30Cx1x^2 - 5Hx1^2x - 30Hx1x^2 + 8x^3 \\
& + Cx1^2 + 2Cx1Hx1 + 9Cx1x + Hx1^2 + 9Hx1x - 6x^2 - Cx1 - Hx1 + x)
\end{aligned}$$

(19)

$$\begin{aligned}
> poss1 := & (4Cx1^4x^6 + 16Cx1^3Hx1x^6 + 24Cx1^2Hx1^2x^6 + 16Cx1Hx1^3x^6 + 4Hx1^4x^6 - \\
& 8Cx1^4x^5 - 32Cx1^3Hx1x^5 - 48Cx1^2Hx1^2x^5 - 32Cx1Hx1^3x^5 - 8Hx1^4x^5 + 8Cx1^4x^4 + \\
& 32Cx1^3Hx1x^4 + 48Cx1^2Hx1^2x^4 + 32Cx1Hx1^3x^4 + 8Hx1^4x^4 - 4Cx1^4x^3 - 16Cx1^3Hx1x^3 + \\
& 12Cx1^3x^4 - 24Cx1^2Hx1^2x^3 + 36Cx1^2Hx1x^4 + 24Cx1^2x^5 - 16Cx1Hx1^3x^3 + \\
& 36Cx1Hx1^2x^4 + 48Cx1Hx1x^5 - 4Hx1^4x^3 + 12Hx1^3x^4 + 24Hx1^2x^5 + Cx1^4x^2 + \\
& 4Cx1^3Hx1x^2 - 16Cx1^3x^3 + 6Cx1^2Hx1^2x^2 - 48Cx1^2Hx1x^3 - 36Cx1^2x^4 + 4Cx1Hx1^3x^2 - \\
& 48Cx1Hx1^2x^3 - 72Cx1Hx1x^4 + Hx1^4x^2 - 16Hx1^3x^3 - 36Hx1^2x^4 + 10Cx1^3x^2 +
\end{aligned}$$

$30Cx1^2Hx1x^2+26Cx1^2x^3+30Cx1Hx1^2x^2+52Cx1Hx1x^3+10Hx1^3x^2+26Hx1^2x^3-$   
 $2Cx1^3x-6Cx1^2Hx1x+Cx1^2x^2-6Cx1Hx1^2x+2Cx1Hx1x^2+36Cx1x^3-$   
 $2Hx1^3x+Hx1^2x^2+36Hx1x^3+4x^4-5Cx1^2x-10Cx1Hx1x-30Cx1x^2-5Hx1^2x-$   
 $30Hx1x^2+8x^3+Cx1^2+2Cx1Hx1+9Cx1x+Hx1^2+9Hx1x-6x^2-Cx1-Hx1+x):$   
 $> poss2 := (16Cx1^4x^{10}+64Cx1^3Hx1x^{10}+96Cx1^2Hx1^2x^{10}+64Cx1Hx1^3x^{10}+$   
 $16Hx1^4x^{10}-32Cx1^4x^9-128Cx1^3Hx1x^9-192Cx1^2Hx1^2x^9-128Cx1Hx1^3x^9-$   
 $32Hx1^4x^9+32Cx1^4x^8+128Cx1^3Hx1x^8+192Cx1^2Hx1^2x^8+128Cx1Hx1^3x^8+$   
 $32Hx1^4x^8-16Cx1^4x^7-64Cx1^3Hx1x^7+48Cx1^3x^8-96Cx1^2Hx1^2x^7+144Cx1^2Hx1x^8+$   
 $96Cx1^2x^9-64Cx1Hx1^3x^7+144Cx1Hx1^2x^8+192Cx1Hx1x^9-16Hx1^4x^7+$   
 $48Hx1^3x^8+96Hx1^2x^9+4Cx1^4x^6+16Cx1^3Hx1x^6-64Cx1^3x^7+24Cx1^2Hx1^2x^6-$   
 $192Cx1^2Hx1x^7-176Cx1^2x^8+16Cx1Hx1^3x^6-192Cx1Hx1^2x^7-352Cx1Hx1x^8+$   
 $4Hx1^4x^6-64Hx1^3x^7-176Hx1^2x^8+40Cx1^3x^6+120Cx1^2Hx1x^6+272Cx1^2x^7+$   
 $120Cx1Hx1^2x^6+544Cx1Hx1x^7+256Cx1x^8+40Hx1^3x^6+272Hx1^2x^7+256Hx1x^8-$   
 $8Cx1^3x^5-24Cx1^2Hx1x^5-260Cx1^2x^6-24Cx1Hx1^2x^5-520Cx1Hx1x^6-336Cx1x^7-$   
 $8Hx1^3x^5-260Hx1^2x^6-336Hx1x^7+16x^8+160Cx1^2x^5+320Cx1Hx1x^5+$   
 $112Cx1x^6+160Hx1^2x^5+112Hx1x^6+192x^7-59Cx1^2x^4-118Cx1Hx1x^4+$   
 $100Cx1x^5-59Hx1^2x^4+100Hx1x^5-256x^6+12Cx1^2x^3+24Cx1Hx1x^3-120Cx1x^4+$   
 $12Hx1^2x^3-120Hx1x^4-124x^5-Cx1^2x^2-2Cx1Hx1x^2+55Cx1x^3-Hx1^2x^2+$   
 $55Hx1x^3+448x^4-12Cx1x^2-12Hx1x^2-365x^3+Cx1x+Hx1x+142x^2-27x+2):$   
 $>$

$> \#$  we use independently calculated initial terms of  $C$  and  $H$  to determine which factor equals 0

```

knownC := x^2*u+108*(1/27+1/54*u)*u*x^3+108*(51907/54+2/27*u
^7+289/108*u^6+949/54*u^5+7295/108*u^4+5111/27*u^3+45329/108*
u^2+13457/18*u)*u*x^9+108*(277/54*u^7+2123/54*u^6+2065/12*u
^5+
59017/108*u^4+74653/54*u^3+26090/9*u^2+271175/54*u+1/12*u
^8+345439/54)*u*x^10+108*(1174607/27+15395/36*u^6+81667/54*u
^5+115144/27*u^4+271756/27*u^3+121663/6*u^2+309613/9*u+5/54*
u^9+269/27*u^8+785/9*u^7)*u*x^11+108*(37661/3*u^5+881623/27*u
^4+439861/6*u^3+7739971/54*u^2+4307179/18*u+11/108*u
^10+2111/108*u^9+20749/108*u^8+18751/18*u^7+12157/3*u
^6+16245425
/54)*u*x^12+108*(18974993/9+13362377/54*u^4+14447794/27*u
^3+55200805/54*u^2+45493075/27*u+1/9*u^11+4171/108*u
^10+7567/18*u^9+67382/27*u^8+95200/9*u^7+106901/3*u
^6+2722970/27*u^5
)*u*x^13+108*(105767759/27*u^3+198363850/27*u^2+323593709/27*u
+13/108*u^12+230/3*u^11+24685/27*u^10+159140/27*u^9+243139/9*
u^8+2651294/27*u^7+899150/3*u^6+42896765/54*u^5+
100716985/54*u^4+403330493/27)*u*x^14+108*(2884113442/27+7/54*u
^13+8243/54*u^12+478427687/9*u^2+773831702/9*u+53383/27*u
^11+123748/9*u^10+1828730/27*u^9+7127600/27*u^8+23303540/
27*u^7+44122847/18*u^6+18543775/3*u^5+378593542/27*u
^4+776849464/27*u^3)*u*x^15+108*(5/36*u^14+32885/108*u
^13+153137/36*u^12+1142381/36*u

```

$^{11+83144798077/108+41789365621/108*u^2+}$   
 $67110072061/108*u+2005483/12*u^{10+25015841/36*u^9+261417547/108*u}$   
 $^{8+263588519/36*u^7+2125739009/108*u^6+5154816665/108*u}$   
 $^{5+11375071513/108*u^4+22901132077/108*u^3)*u*x^{16+108*(4}$   
 $/27*u^{15+65669/108*u^{14+491917/54*u^{13+7835237/108*u}$   
 $^{12+10980847/27*u^{11+64661717/36*u^{10+244061356147/54*u}$   
 $+358364017/54*u^9+2298037063/108*u^8+1637272894/27*u}$   
 $^{7+16858482193/108}$   
 $*u^6+733571455/2*u^5+85456504375/108*u^4+1568029281*u$   
 $^{3+101936028323/36*u^2+11172727177/2)*u*x^{17+108*(65611/54*u}$   
 $^{15+116561/6*u^{14+17764891/108*u^{13+105597419/108*u}$   
 $^{12+246760037}$   
 $/54*u^{11+481708913/27*u^{10+2174181161/36*u^9+19619913763/108*u}$   
 $^{8+1481546501/3*u^7+66281718671/54*u^6+303513226133/108*u}$   
 $^{5+642510529985/108*u^4+209391918407/18*u^3+562149075844/}$   
 $27*u^2+1785210018043/54*u^{17/108*u^{16+2202060528251/54})*u*x$   
 $^{18+108*(39982715/108*u^{14+41859775/18*u^{13+309533033/27*u}$   
 $^{12+1272898912/27*u^{11+18136104811/108*u^{10+1062491085/2*u^9}$   
 $+82021550137/54*u^8+8079669856907/27+107292067916/27*u}$   
 $^{7+1036223152901/108*u^6+386921648897/18*u}$   
 $^{5+1209106114540/27*u^4+779129791984/9*u^3+8302736243227/54*u}$   
 $^{2+2187273831257/9*u}$   
 $+1/6*u^{17+65578/27*u^{16+1114391/27*u^{15})*u*x}$   
 $^{19+108*(119139609551851/54+511310599/18*u^{13+6625377505/54*u}$   
 $^{12+49522083229/108*u^{11+164268802187/108*u}$   
 $^{10+492349769597/108*u^9+}$   
 $1350678393421/108*u^8+1711569280457/54*u^7+2016613040566/27*u}$   
 $^{6+4435356872482/27*u^5+9114089718610/27*u}$   
 $^{4+11630360068117/18*u^3+61554977870293/54*u}$   
 $^{2+96909115204843/54*u+19/108*}$   
 $u^{18+19425/4*u^{17+1048721/12*u^{16+22349542/27*u^{15+295845395/54*u}$   
 $^{14})*u*x^{20+108*(133061611057/108*u^{12+38466297097/9*u}$   
 $^{11+482095357475/36*u^{10+76807868977/2*u^9+2748472831498/}$   
 $27*u^8+2260582751408/9*u^7+5217654402278/9*u}$   
 $^{6+147016196120819/9+33885035327588/27*u^5+45869809116205/18*}$   
 $u^4+14507532710398/3*u^3+152662877430509/18*u}$   
 $^{2+359248731055321/27*u+5/}$   
 $27*u^{19+1048783/108*u^{18+3320743/18*u^{17+99356867/54*u}$   
 $^{16+345515888/27*u^{15+139216063/2*u^{14+314988459*u^{13})*u*x}$   
 $^{21+108*(694689967903/18*u^{11+3115838996140/27*u}$   
 $^{10+8612771898950}$   
 $/27*u^9+22176293556902/27*u^8+1980839503368*u}$   
 $^{7+121256513931676/27*u}$   
 $^{6+3277895968713443/27+517788614853439/54*u}$   
 $^{5+1040475128140955/54*u^4+326580948503611/9*u}$   
 $^{3+1709353913764874/}$



$27*u^2+2673249306766819/27*u+7/36*u^{20}+524345/27*u$   
 $\quad \quad \quad ^{19}+10486196/27*u^{18}+24409093/6*u^{17}+1601725207/54*u$   
 $\quad \quad \quad ^{16}+4559655350/27*u^{15}+21568885061/27*u^{14}+117465620455/36*u$   
 $\quad \quad \quad ^{13}+$   
 $1275582417361/108*u^{12})*u*x^{22}+108*(26409329661782/27*u$   
 $\quad \quad \quad ^{10}+7862433511660/3*u^9+177727586499748/27*u$   
 $\quad \quad \quad ^8+46693797793696/3*u^7+1876121436483583/54*u$   
 $\quad \quad \quad ^6+659580878781871/9*u^5+$   
 $3939743341223870/27*u^4+2456520646796824/9*u$   
 $\quad \quad \quad ^3+12797854294664491/27*u^2+6652762259157082/9*u+11/54*u$   
 $\quad \quad \quad ^{21}+2097277/54*u^{20}+22020595/27*u^{19}+483399701/54*u$   
 $\quad \quad \quad ^{18}+614470793/9*u^{17}+$   
 $24445469953511182/27+3654223139/9*u^{16}+54100238644/27*u$   
 $\quad \quad \quad ^{15}+307063989671/36*u^{14}+192908249891/6*u$   
 $\quad \quad \quad ^{13}+2952151225964/27*u^{12}+9183814752128/27*u^{11})*u*x$   
 $\quad \quad \quad ^{23}+108*(576400699485595/27*u$   
 $\quad \quad \quad ^9+1416892254175387/27*u^8+243928948120431/2*u$   
 $\quad \quad \quad ^7+14501462340215887/54*u^6+30263459077896139/54*u$   
 $\quad \quad \quad ^5+59763916058790235/54*u^4+4115514794219043/2*u$   
 $\quad \quad \quad ^3+192161294136410573/54*u^2+$   
 $298917494561253353/54*u+184551647/108*u^{20}+2118138125/108*u$   
 $\quad \quad \quad ^{19}+16865374093/108*u^{18}+34855483867/36*u$   
 $\quad \quad \quad ^{17}+537367278713/108*u^{16}+23/108*u^{22}+8388881/108*u$   
 $\quad \quad \quad ^{21}+365757121431153641/54+$   
 $1189873711343/54*u^{15}+2331108073985/27*u^{14}+8235401655821/27*u$   
 $\quad \quad \quad ^{13}+26603007578101/27*u^{12}+79421612769499/27*u$   
 $\quad \quad \quad ^{11}+220945335244663/27*u^{10})*u*x^{24}+108*(2499841927753457/6*u$   
 $\quad \quad \quad ^8+$   
 $2861216996699140/3*u^7+37343944843007665/18*u$   
 $\quad \quad \quad ^6+115790925300927799/27*u^5+151327723052351669/18*u$   
 $\quad \quad \quad ^4+139919154160874066/9*u$   
 $\quad \quad \quad ^3+457352335125595381/9+160702678767780461/6*u^2+$   
 $1122338903556212447/27*u+3196067557/9*u^{19}+247485358253/108*u$   
 $\quad \quad \quad ^{18}+220369746229/18*u^{17}+1520427021667/27*u$   
 $\quad \quad \quad ^{16}+2060879608048/9*u^{15}+2/9*u^{23}+16777513/108*u$   
 $\quad \quad \quad ^{22}+192939269/54*u^{21}+$   
 $4622140187/108*u^{20}+7551142961023/9*u^{14}+25286468986270/9*u$   
 $\quad \quad \quad ^{13}+234702539623237/27*u^{12}+75177002785708/3*u$   
 $\quad \quad \quad ^{11}+609798116835341/9*u^{10}+4663181417105186/27*u^9)*u*x$   
 $\quad \quad \quad ^{25}+108*($   
 $8449572374778841259/27*u+1898205696572318/9*u^{11}+25/108*u$   
 $\quad \quad \quad ^{24}+1773425621107004441/54*u^5+3453664462468926469/54*u$   
 $\quad \quad \quad ^4+1059214428869797967/9*u^3+5455740584680732108/27*u^2+$   
 $432647929591107581/27*u^6+682643187354071/27*u$   
 $\quad \quad \quad ^{13}+2035828889737523/27*u^{12}+15020981418524764/27*u$   
 $\quad \quad \quad ^{10}+1864153/6*u^{23}+75039163825511089/54*u$

^9+178043368303673465/54\*u^8+  
67018337256808130/9\*u^7+427488040943/3\*u  
^17+10321065261320737963/27+3349857487/36\*u  
^21+86755098941/108\*u^20+290862682405/54\*u  
^19+16212663883171/27\*u^16+20506500741952/9\*u^15+  
806540107496/27\*u^18+402654631/54\*u^22+213238259393794/27\*u^14)\*u  
\*x^26+108\*(63762893957419461254/27\*u+47459727187464080/27\*u  
^11+16777303/27\*u^24+13/54\*u^25+6795736852184881271/  
27\*u^5+1461723337560575812/3\*u^4+24100410127831033136/27\*u  
^3+41249271763722688987/27\*u^2+2227645384584934307/18\*u  
^6+6028531594804346/27\*u^13+5805921532112284/9\*u^12+  
244997819805642065/54\*u^10+419431211/27\*u  
^23+300542464593698213/27\*u^9+702653959186060267/27\*u  
^8+1567960838790253160/27\*u^7+42072865444550/27\*u  
^17+77826943776337392262/27+  
97643466295/54\*u^21+339684274118/27\*u^20+650921291708/9\*u  
^19+165111841899046/27\*u^16+591588275693968/27\*u  
^15+9647546214839/27\*u^18+21776849693/108\*u  
^22+1956874412461303/27\*u^14)  
\*u\*x^27+108\*(482222978602732258409/27\*u+784690311600145301/54\*u  
^11+3489664549/108\*u^24+134218103/108\*u  
^25+588178017425067244649/27+52125273452289026642/27\*u^5+  
100359511360520975746/27\*u^4+183107769613435259741/27\*u  
^3+104168348607659270305/9\*u^2+2867751940097458430/3\*u  
^6+52427872817036146/27\*u^13+49115774717538422/9\*u^12+  
1986860508830698591/54\*u^10+2613518923/6\*u  
^23+4797479209683216437/54\*u^9+1/4\*u  
^26+1229927159344415005/6\*u^8+4072563269055131261/9\*u  
^7+146119584010567/9\*u^17+788772639056/27\*u^21  
+521588844346/3\*u^20+23989388840413/27\*u^19+1621535178416077/27\*u  
^16+205010505138236\*u^15+108135107998735/27\*u  
^18+109404266866/27\*u^22+17592345855170846/27\*u^14)\*u\*x  
^28+108\*(  
3654319522465156336438/27\*u+3221751848279417678/27\*u  
^11+8444534635/9\*u^24+1207960223/18\*u  
^25+4454407600151505824566/27+400151655665151913252/27\*u  
^5+766616904794131813505/27\*u^4+  
1393498476535079871076/27\*u^3+2372008466176074589901/27\*u  
^2+199399217954034536866/27\*u^6+450200886444301012/27\*u  
^13+2469782396866423997/54\*u^12+16038464845214048977/54\*u^10+  
244142096312/27\*u^23+19088587638130539755/27\*u^9+268435859/108\*u  
^26+43524048354998657378/27\*u^8+95144186528774901584/27\*u  
^7+4395246883069646/27\*u^17+11210285347504/27\*u^21+  
19729686277091/9\*u^20+275459258895140/27\*u^19+572807911602998\*u  
^16+50650503791767072/27\*u^15+1152176707222681/27\*u  
^18+1821687157024/27\*u^22+7/27\*u^27+155506245583438610/27\*u

$^{14})$   
 $*u*x^{29+108*(9248297084729193568478/9*u+8769063296949931315/9*u^{11+180903147038/9*u^{24+6047255285/3*u^{25+29/108*u^{28+33799474943774797568666/27+1024814891971863907583/9*u^{5+651479232300231209113/3*u^{4+3540464674773182594746/9*u^{3+6011996014045069168588/9*u^{2+1540961166604170540668/27*u^{6+7650440008456709189/54*u^{13+20537447590203799649/54*u^{12+21494791893740045228/9*u^{10+1395361162886/9*u^{23+5612316773800624786*u^{9+3758097499/27*u^{26+341821527903730776502/27*u^{8+82291605071042621080/3*u^{7+42722376525692878/27*u^{17+48328255033135/9*u^{21+695903261477917/27*u^{20+3000256598738518/27*u^{19+144023381758608446/27*u^{16+45503586652729552/27*u^{15+3930250035487364/9*u^{18+26606652909256/27*u^{22+134217836/27*u^{27+1355437625261588996/27*u^{14})}*x^{30+108*(7/108*u^{6+17/12*u^{5+839/108*u^{4+923/36*u^{3+6665/108*u^{2+12341/108*u^{16061/108})}*x^{8+108*(647/27+1/18*u^{5+41/54*u^{4+91/27*u^{3+499/54*u^{2+163/9*u})}*x^{7+108*(5/108*u^{4+11/27*u^{3+38/27*u^{2+163/54*u^{221/54})}*x^{6+108*(1/27*u^{3+29/54*u^{41/54+23/108*u^{2})}*x^{5+108*(1/36*u^{2+11/108*u^{17/108})}*x^{4:}$

$\text{knownH} := x+(u+2)*x^2+(u^2+4*u+6)*x^3+(u^3+8*u^2+18*u+24)*x^4+(u^4+16*u^3+50*u^2+92*u+116)*x^5+(u^5+32*u^4+130*u^3+308*u^2+516*u+632)*x^6+(u^6+64*u^5+322*u^4+932*u^3+1940*u^2+3088*u+3720)$

$*x^7+(u^7+128*u^6+770*u^5+2628*u^4+6484*u^3+12544*u^2+19352*u+23072)*x^8+(u^8+256*u^7+1794*u^6+7044*u^5+19988*u^4+44960*u^3+83032*u^2+125456*u+148528)*x^9+(u^9+512*u^8+4098*u^7+18180*u^6+58132*u^5+147936*u^4+313368*u^3+560560*u^2+834544*u+983072)*x^{10}+(u^{10}+1024*u^9+9218*u^8+45572*u^7+161812*u^6+457568*u^5+1083672*u^4+2201072*u^3+3847088*u^2+5664704*u+6647776)*x^{11}+(u^{11}+2048*u^{10}+20482*u^9+111620*u^8+435220*u^7+1350240*u^6+3516952*u^5+7915376*u^4+15586480*u^3+26767360*u^2+39079840*u+45727616)*x^{12}+(u^{12}+4096*u^{11}+45058*u^{10}+268292*u^9+1138708*u^8+3839072*u^7+10872344*u^6+26699376*u^5+57849264*u^4+111235456*u^3+188412064*u^2+273219520*u+318947136)*x^{13}+(u^{13}+8192*u^{12}+98306*u^{11}+634884*u^{10}+2912276*u^9+10590304*u^8+32334360*u^7+85729392*u^6+201404848*u^5+423727232*u^4+799568288*u^3+1339359552*u^2+1931526208*u+2250473344)*x^{14}+(u^{14}+16384*u^{13}+212994*u^{12}+1482756*u^{11}+7307284*u^{10}+28487776*u^9+93155864*u^8+264610928*u^7+667397552*u^6+1514703488*u^5+3112856992*u^4+5784928320*u^3+9602253120*u^2+13784252672*u+16034726016)*x^{15}+(u^{15}+32768*u^{14}+$

458754\*u<sup>13</sup>+3424260\*u<sup>12</sup>+18038804\*u<sup>11</sup>+75014240\*u<sup>10</sup>+261325336\*u<sup>9</sup>+790543472\*u<sup>8</sup>+2125315504\*u<sup>7</sup>+5154573952\*u<sup>6</sup>+11379304864\*u<sup>5</sup>+22942513728\*u<sup>4</sup>+42101292352\*u<sup>3</sup>+69350850560\*u<sup>2</sup>+  
99169829248\*u+115204555264)\*x<sup>16</sup>+(u<sup>16</sup>+65536\*u<sup>15</sup>+983042\*u<sup>14</sup>+7831556\*u<sup>13</sup>+43909140\*u<sup>12</sup>+193937504\*u<sup>11</sup>+716587544\*u<sup>10</sup>+2297670768\*u<sup>9</sup>+6548278704\*u<sup>8</sup>+16857278080\*u<sup>7</sup>+39614904736\*  
u<sup>6</sup>+85493284416\*u<sup>5</sup>+169650141504\*u<sup>4</sup>+308032895488\*u<sup>3</sup>+504122080640\*u<sup>2</sup>+718496465152\*u+833701020416)\*x<sup>17</sup>+(u<sup>17</sup>+131072\*u<sup>16</sup>+2097154\*u<sup>15</sup>+17760260\*u<sup>14</sup>+105578516\*u<sup>13</sup>+493453408\*u<sup>12</sup>+1926627864\*u<sup>11</sup>+6521965680\*u<sup>10</sup>+19618500016\*u<sup>9</sup>+53332907648\*u<sup>8</sup>+132561734048\*u<sup>7</sup>+303541655104\*u<sup>6</sup>+642796210496\*u<sup>5</sup>+1258543054336\*u<sup>4</sup>+2264536742272\*u<sup>3</sup>+3685494946560\*u<sup>2</sup>+  
5237692432128\*u+6071393452544)\*x<sup>18</sup>+(u<sup>18</sup>+262144\*u<sup>17</sup>+4456450\*u<sup>16</sup>+39976964\*u<sup>15</sup>+251133972\*u<sup>14</sup>+1238040672\*u<sup>13</sup>+5091295768\*u<sup>12</sup>+18135223408\*u<sup>11</sup>+57372200368\*u<sup>10</sup>+164037867136\*u<sup>9</sup>+429160352160\*u<sup>8</sup>+1036237014592\*u<sup>7</sup>+2321783707968\*u<sup>6</sup>+4838550869504\*u<sup>5</sup>+9365373880704\*u<sup>4</sup>+16720329047808\*u<sup>3</sup>+27080509356800\*u<sup>2</sup>+38389595241472\*u+44460988694016)\*x<sup>19</sup>+(  
u<sup>19</sup>+524288\*u<sup>18</sup>+9437186\*u<sup>17</sup>+89391108\*u<sup>16</sup>+591659028\*u<sup>15</sup>+3067740256\*u<sup>14</sup>+13250331160\*u<sup>13</sup>+49520774256\*u<sup>12</sup>+164265151920\*u<sup>11</sup>+492340737664\*u<sup>10</sup>+1350660458912\*u<sup>9</sup>+3423127840320\*u<sup>8</sup>+  
8066649528640\*u<sup>7</sup>+17743432320512\*u<sup>6</sup>+36471929608576\*u<sup>5</sup>+69896552978176\*u<sup>4</sup>+123942367136512\*u<sup>3</sup>+199887856599040\*u<sup>2</sup>+282738440534528\*u+327199429228544)\*x<sup>20</sup>+(u<sup>20</sup>+1048576\*u<sup>19</sup>+  
19922946\*u<sup>18</sup>+198705156\*u<sup>17</sup>+1382023188\*u<sup>16</sup>+7517503584\*u<sup>15</sup>+34018165272\*u<sup>14</sup>+133059710064\*u<sup>13</sup>+461589990832\*u<sup>12</sup>+1446271317632\*u<sup>11</sup>+4147591252384\*u<sup>10</sup>+10993840285248\*u<sup>9</sup>+  
27127093614912\*u<sup>8</sup>+62613639308800\*u<sup>7</sup>+135555248052608\*u<sup>6</sup>+275332319282944\*u<sup>5</sup>+523101849000704\*u<sup>4</sup>+922043861178368\*u<sup>3</sup>+1481449348794880\*u<sup>2</sup>+2091387218557952\*u+2418586647786496)\*  
x<sup>21</sup>+(u<sup>21</sup>+2097152\*u<sup>20</sup>+41943042\*u<sup>19</sup>+439353348\*u<sup>18</sup>+3203399700\*u<sup>17</sup>+18238406752\*u<sup>16</sup>+86274736664\*u<sup>15</sup>+352394153072\*u<sup>14</sup>+1275574111664\*u<sup>13</sup>+4168116598400\*u<sup>12</sup>+12463298120096\*u<sup>11</sup>+  
34450972042816\*u<sup>10</sup>+88705113545024\*u<sup>9</sup>+213932073215488\*u<sup>8</sup>+485040318847360\*u<sup>7</sup>+1035688922687232\*u<sup>6</sup>+2081777416133376\*u<sup>5</sup>+3925031437469696\*u<sup>4</sup>+6881858741606912\*u<sup>3</sup>+  
11020172190028800\*u<sup>2</sup>+15530146056373248\*u+17948732704159744)\*x<sup>22</sup>+(u<sup>22</sup>+4194304\*u<sup>21</sup>+88080386\*u<sup>20</sup>+966787076\*u<sup>19</sup>+7373586452\*u<sup>18</sup>+43850399840\*u<sup>17</sup>+216399872536\*u<sup>16</sup>+921188174960\*  
u<sup>15</sup>+3472336375216\*u<sup>14</sup>+11808569423488\*u<sup>13</sup>+36735164680608\*u<sup>12</sup>

$^{12}+105637102118464*u^{11}+283047283480896*u$   
 $^{10}+710911110964736*u^9+1680989498186112*u$   
 $^8+3752351308834560*u^7+$   
 $7915790936546048*u^6+15765020110465024*u^5+29522666200226304*u$   
 $^4+51518549591589888*u^3+82251642275107840*u$   
 $^2+115730521035640832*u+133679253739800576)*x^{23}+(u$   
 $^{23}+8388608*u^{22}+$   
 $184549378*u^{21}+2118123524*u^{20}+16865296404*u^{19}+104566095968*u$   
 $^{18}+537365840408*u^{17}+2379742186608*u^{16}+9324414913968*u$   
 $^{15}+32941553612416*u^{14}+106411881990560*u^{13}+$   
 $317686079579712*u^{12}+883780600813888*u^{11}+2305602503796224*u$   
 $^{10}+5667579249695104*u^9+13172265832638208*u$   
 $^8+29003732501175040*u^7+60532939021084672*u$   
 $^6+119572200028084736*u^5+$   
 $222564838222570496*u^4+386740923343557632*u^3+615783378767052800*$   
 $u^2+865193153542494208*u+998872407282294784)*x^{24}+(u$   
 $^{24}+16777216*u^{23}+385875970*u^{22}+4622123012*u^{21}+38352715796$   
 $*u^{20}+247484907616*u^{19}+1322216587800*u^{18}+6081700957296*u$   
 $^{17}+24730530762160*u^{16}+90613637838464*u^{15}+303437400836512*u$   
 $^{14}+938809553348160*u^{13}+2706370709248320*u^{12}+$   
 $7317575397893632*u^{11}+18652731646810496*u^{10}+44997247277360896*u$   
 $^9+103004597075155712*u^8+224069641416304640*u$   
 $^7+463207970079021568*u^6+908293185535468544*u^5+$   
 $1681447832793355264*u^4+2910596003679674368*u$   
 $^3+46223033578060503040*u^2+6487099138885292032*u$   
 $+7485971546167586816)*x^{25}+(u^{25}+33554432*u^{24}+805306370*u$   
 $^{23}+10049552388*u^{22}+$   
 $86754983956*u^{21}+581724799072*u^{20}+3226157974040*u$   
 $^{19}+15389559884912*u^{18}+64850621386160*u^{17}+246077896914560*u$   
 $^{16}+852952697604512*u^{15}+2730571797653056*u$   
 $^{14}+8143313170422080*u^{13}+$   
 $13+22778463647262208*u^{12}+60083924690409856*u$   
 $^{11}+150078403210405632*u^{10}+356087482156161792*u$   
 $^9+804225931287750656*u^8+1730635800052341248*u$   
 $^7+3547177710134584320*u^6+$   
 $6909746176292066304*u^5+12728519597003628544*u$   
 $^4+21956638020420474880*u^3+34797157044451258368*u$   
 $^2+48770227729504137216*u+56256199275671724032)*x^{26}+(u$   
 $^{26}+67108864*u^{25}+$   
 $1677721602*u^{24}+21776826372*u^{23}+195286794260*u^{22}+1358736392288*$   
 $u^{21}+7811052339736*u^{20}+38590172105840*u^{19}+168291414855088*u$   
 $^{18}+660447208535680*u^{17}+2366352602761632*u^{16}+$   
 $7827496191419968*u^{15}+24114122486536512*u^{14}+69671049462113792*u$   
 $^{13}+189838896592460160*u^{12}+489995686978545408*u$   
 $^{11}+1202170536086313728*u^{10}+2810621564960794624*u^9+$   
 $6271887093672024576*u^8+13366198052952499200*u$

$^7+27185363206107403264*u^6+52639983813466873856*u$   
 $^5+96535311121603663872*u^4+165995945956766380032*u$   
 $^3+262537529008492359680*u^2+$   
 $367563956013668220928*u+423820155289339944960)*x^{27}+(u$   
 $^{27}+134217728*u^{26}+3489660930*u^{25}+47043313668*u$   
 $^{24}+437616902164*u^{23}+3155089686624*u^{22}+18777194365464*u$   
 $^{21}+95957538573424$   
 $*u^{20}+432540368260528*u^{19}+1753434785183360*u$   
 $^{18}+6486139989723552*u^{17}+22141132365915712*u$   
 $^{16}+70369377293261120*u^{15}+209711475898541568*u$   
 $^{14}+589389266832988544*u^{13}+$   
 $1569380624755353344*u^{12}+3973721581723425536*u$   
 $^{11}+9594963877943994368*u^{10}+22138731993894590976*u$   
 $^9+48871083638810895360*u^8+103241482851596473344*u$   
 $^7+208519031891882434560*u^6+$   
 $401571705402385602560*u^5+733429918062178562048*u$   
 $^4+1257506103671880986624*u^3+1985148044153049841664*u$   
 $^2+2776532155456058007552*u+3200352310745397952512)*x^{28}+(u$   
 $^{28}+268435456*u$   
 $^{27}+7247757314*u^{26}+101334384644*u^{25}+976568188948*u$   
 $^{24}+7286747562080*u^{23}+44841136292376*u^{22}+236756213435504*u$   
 $^{21}+1101836949933488*u^{20}+4608706520151680*u$   
 $^{19}+17580986498615712$   
 $*u^{18}+61863251223799360*u^{17}+202602005764593984*u$   
 $^{16}+622024957242729984*u^{15}+1800803488658233728*u$   
 $^{14}+4939564722134214400*u^{13}+12887007770376510208*u$   
 $^{12}+32076934692563478528*u^{11}+$   
 $11+76354392608959207936*u^{10}+174096515425592304640*u$   
 $^9+380579153929356022784*u^8+797614799126473105408*u$   
 $^7+1600740261198540150784*u^6+3067466418069157474304*u^5+$   
 $5581479753005637152768*u^4+9544289869765569249280*u$   
 $^3+15041097981402013540352*u^2+21017982447603469500416*u$   
 $+24218334758348867452928)*x^{29}+(u^{29}+536870912*u$   
 $^{28}+15032385538*u^{27}+$   
 $217701154820*u^{26}+2170837532692*u^{25}+16744332656736*u$   
 $^{24}+106426605240856*u^{23}+579939032108144*u$   
 $^{22}+2783612931952048*u^{21}+12001025972106880*u$   
 $^{20}+47162998968355232*u^{19}+$   
 $170889501409306176*u^{18}+576093512892766528*u$   
 $^{17}+1820143427059279360*u^{16}+5421750402125273472*u$   
 $^{15}+15300879830358976256*u^{14}+41074895255907441408*u$   
 $^{13}+105228763807333378048*u^{12}+$   
 $257937542953858341376*u^{11}+606130529344054256640*u$   
 $^{10}+1367288510003337073664*u^9+2962515689669635497984*u$   
 $^8+6163978263334011639808*u^7+12298777420218586787840*u^6+$   
 $23460738053822578798592*u^5+42541831821807549710336*u$

```

^4+72567771585335905067008*u^3+114179916325253504122880*u
^2+159416233531205841076224*u+183634568289554708529152)*x^30:

```

```

>
> series(subs({ Cx1 = subs(u = 1, knownC), Hx1 = subs(u = 1, knownH)}, poss1), x, 40)

```

$$\begin{aligned}
& 7825352008549467248813597x^{31} \\
& - 26400099623526437042868665x^{32} \\
& + 49748120832505414249409412x^{33} \\
& + 178512812456673652234628216x^{34} \\
& + 1102677336134614596424073946x^{35} \\
& + 7574742227008772053960734316x^{36} \\
& + 51776685679776930442389402208x^{37} \\
& + 355035402174837270111769272008x^{38} \\
& + 2441323675505092350943577926846x^{39} + O(x^{40})
\end{aligned} \tag{20}$$

```

> series(subs({ Cx1 = subs(u = 1, knownC), Hx1 = subs(u = 1, knownH)}, poss2), x, 21)

```

$$\begin{aligned}
& 2 - 27x + 143x^2 - 373x^3 + 471x^4 - 142x^5 - 256x^6 \\
& + 446x^7 + 1136x^8 + 8282x^9 + 58740x^{10} + 419758x^{11} \\
& + 3021276x^{12} + 21885036x^{13} + 159429920x^{14} + 1167369484x^{15} \\
& + 8587161800x^{16} + 63432089882x^{17} + 470353988796x^{18} \\
& + 3499893261694x^{19} + 26126011379100x^{20} + O(x^{21})
\end{aligned} \tag{21}$$

```

>
> # therefore poss1 is the correct factor
> new_eq3 := poss1

```

$$\begin{aligned}
new\_eq3 := & 4Cx1^4x^6 + 16Cx1^3Hx1x^6 \\
& + 24Cx1^2Hx1^2x^6 + 16Cx1Hx1^3x^6 \\
& + 4Hx1^4x^6 - 8Cx1^4x^5 - 32Cx1^3Hx1x^5 \\
& - 48Cx1^2Hx1^2x^5 - 32Cx1Hx1^3x^5 - 8Hx1^4x^5 \\
& + 8Cx1^4x^4 + 32Cx1^3Hx1x^4 + 48Cx1^2Hx1^2x^4 \\
& + 32Cx1Hx1^3x^4 + 8Hx1^4x^4 - 4Cx1^4x^3 \\
& - 16Cx1^3Hx1x^3 + 12Cx1^3x^4 - 24Cx1^2Hx1^2x^3 \\
& + 36Cx1^2Hx1x^4 + 24Cx1^2x^5 - 16Cx1Hx1^3x^3 \\
& + 36Cx1Hx1^2x^4 + 48Cx1Hx1x^5 - 4Hx1^4x^3 \\
& + 12Hx1^3x^4 + 24Hx1^2x^5 + Cx1^4x^2 \\
& + 4Cx1^3Hx1x^2 - 16Cx1^3x^3 + 6Cx1^2Hx1^2x^2 \\
& - 48Cx1^2Hx1x^3 - 36Cx1^2x^4 + 4Cx1Hx1^3x^2 \\
& - 48Cx1Hx1^2x^3 - 72Cx1Hx1x^4 + Hx1^4x^2 \\
& - 16Hx1^3x^3 - 36Hx1^2x^4 + 10Cx1^3x^2 \\
& + 30Cx1^2Hx1x^2 + 26Cx1^2x^3 + 30Cx1Hx1^2x^2 \\
& + 52Cx1Hx1x^3 + 10Hx1^3x^2 + 26Hx1^2x^3 \\
& - 2Cx1^3x - 6Cx1^2Hx1x + Cx1^2x^2 \\
& - 6Cx1Hx1^2x + 2Cx1Hx1x^2 + 36Cx1x^3 \\
& - 2Hx1^3x + Hx1^2x^2 + 36Hx1x^3 + 4x^4 \\
& - 5Cx1^2x - 10Cx1Hx1x - 30Cx1x^2 - 5Hx1^2x \\
& - 30Hx1x^2 + 8x^3 + Cx1^2 + 2Cx1Hx1 + 9Cx1x \\
& + Hx1^2 + 9Hx1x - 6x^2 - Cx1 - Hx1 + x
\end{aligned} \tag{22}$$

```

>
> eqs := eqs union {new_eq3}:
>
>
> PI := PolynomialIdeal(eqs, parameters = {x, u}):
> HilbertDimension(PI)

```

$$1 \tag{23}$$

```

>
> Bans := factor(Generators(EliminationIdeal(PI, {Bx1}))[1])

```



$$\begin{aligned}
Bans := & (16Bx1^4x^6 - 32Bx1^4x^5 \\
& - 128Bx1^3x^6 + 32Bx1^4x^4 + 256Bx1^3x^5 \\
& + 384Bx1^2x^6 - 16Bx1^4x^3 - 264Bx1^3x^4 \\
& - 736Bx1^2x^5 - 512Bx1x^6 + 4Bx1^4x^2 \\
& + 152Bx1^3x^3 + 744Bx1^2x^4 \\
& + 896Bx1x^5 + 256x^6 - 52Bx1^3x^2 \\
& - 444Bx1^2x^3 - 832Bx1x^4 - 384x^5 \\
& + 8Bx1^3x + 169Bx1^2x^2 + 456Bx1x^3 \\
& + 304x^4 - 38Bx1^2x - 154Bx1x^2 \\
& - 136x^3 + 4Bx1^2 + 29Bx1x + 29x^2 \\
& - 2Bx1 - 2x) (16Bx1^4x^7 - 32Bx1^4x^6 \\
& - 128Bx1^3x^7 + 32Bx1^4x^5 + 256Bx1^3x^6 \\
& + 320Bx1^2x^7 - 16Bx1^4x^4 - 264Bx1^3x^5 \\
& - 608Bx1^2x^6 - 256Bx1x^7 + 4Bx1^4x^3 \\
& + 152Bx1^3x^4 + 620Bx1^2x^5 \\
& + 384Bx1x^6 + 64x^7 - 52Bx1^3x^3 \\
& - 388Bx1^2x^4 - 288Bx1x^5 - 32x^6 \\
& + 8Bx1^3x^2 + 161Bx1^2x^3 + 140Bx1x^4 \\
& - 108x^5 - 42Bx1^2x^2 - 54Bx1x^3 \\
& + 184x^4 + 5Bx1^2x + 25Bx1x^2 \\
& - 138x^3 - 8Bx1x + 57x^2 + Bx1 - 12x \\
& + 1) (4Bx1^4x^6 - 8Bx1^4x^5 + 8Bx1^4x^4 \\
& + 12Bx1^3x^5 - 4Bx1^4x^3 - 28Bx1^3x^4 \\
& + 12Bx1^2x^5 + Bx1^4x^2 + 26Bx1^3x^3 \\
& - 5Bx1^2x^4 - 12Bx1^3x^2 - 16Bx1^2x^3 \\
& + 18Bx1x^4 + 2Bx1^3x + 21Bx1^2x^2 \\
& - 27Bx1x^3 + x^4 - 8Bx1^2x + 10Bx1x^2 \\
& + Bx1^2 - Bx1x) (16Bx1^4x^7 \\
& - 32Bx1^4x^6 + 32Bx1^4x^5 + 48Bx1^3x^6 \\
& - 64Bx1^2x^7 - 16Bx1^4x^4 - 112Bx1^3x^5 \\
& + 176Bx1^2x^6 + 4Bx1^4x^3 \\
& + 104Bx1^3x^4 - 144Bx1^2x^5 \\
& - 32Bx1x^6 + 64x^7 - 48Bx1^3x^3 \\
& - 8Bx1^2x^4 + 208Bx1x^5 - 128x^6 \\
& + 8Bx1^3x^2 + 76Bx1^2x^3 - 252Bx1x^4 \\
& + 192x^5 - 36Bx1^2x^2 + 108Bx1x^3 \\
& - 84x^4 + 5Bx1^2x - 6Bx1x^2 - 37x^3 \\
& - 6Bx1x + 40x^2 + Bx1 - 11x + 1)
\end{aligned} \tag{24}$$

```

>
> # we need to determine which factor of Bans is the correct minimal polynomial for B(x, 1)
>
> qq := sort(factors(Bans)[2])

```

$$\begin{aligned}
qq := & \left[ \left[ Bx1^4x^6 - 2Bx1^4x^5 + 2Bx1^4x^4 + 3Bx1^3x^5 - Bx1^4x^3 - 7Bx1^3x^4 \right. \right. \quad (25) \\
& + 3Bx1^2x^5 + \frac{1}{4}Bx1^4x^2 + \frac{13}{2}Bx1^3x^3 - \frac{5}{4}Bx1^2x^4 - 3Bx1^3x^2 - 4Bx1^2x^3 \\
& + \frac{9}{2}Bx1x^4 + \frac{1}{2}Bx1^3x + \frac{21}{4}Bx1^2x^2 - \frac{27}{4}Bx1x^3 + \frac{1}{4}x^4 - 2Bx1^2x + \frac{5}{2}Bx1x^2 \\
& + \frac{1}{4}Bx1^2 - \frac{1}{4}Bx1x, 1 \left. \right], \left[ -\frac{1}{8}x - \frac{77}{8}Bx1x^2 - \frac{17}{2}x^3 + 16x^6 - 24x^5 - \frac{1}{8}Bx1 \right. \\
& + \frac{29}{16}Bx1x + \frac{29}{16}x^2 + \frac{1}{4}Bx1^4x^2 + \frac{1}{4}Bx1^2 + 19x^4 + Bx1^4x^6 - 2Bx1^4x^5 \\
& - 8Bx1^3x^6 + 2Bx1^4x^4 + 16Bx1^3x^5 + 24Bx1^2x^6 - Bx1^4x^3 - \frac{33}{2}Bx1^3x^4 \\
& - 46Bx1^2x^5 - 32Bx1x^6 + \frac{19}{2}Bx1^3x^3 + \frac{93}{2}Bx1^2x^4 + 56Bx1x^5 - \frac{13}{4}Bx1^3x^2 \\
& - \frac{111}{4}Bx1^2x^3 - 52Bx1x^4 + \frac{1}{2}Bx1^3x + \frac{169}{16}Bx1^2x^2 + \frac{57}{2}Bx1x^3 \\
& - \frac{19}{8}Bx1^2x, 1 \left. \right], \left[ -\frac{11}{16}x + 4x^7 - \frac{3}{8}Bx1x^2 - \frac{37}{16}x^3 - 8x^6 + 12x^5 + \frac{1}{16}Bx1 \right. \\
& - \frac{3}{8}Bx1x + \frac{5}{2}x^2 + \frac{1}{16} - \frac{21}{4}x^4 + Bx1^4x^7 - 2Bx1^4x^6 + 2Bx1^4x^5 + 3Bx1^3x^6 \\
& - 4Bx1^2x^7 - Bx1^4x^4 - 7Bx1^3x^5 + 11Bx1^2x^6 + \frac{1}{4}Bx1^4x^3 + \frac{13}{2}Bx1^3x^4 \\
& - 9Bx1^2x^5 - 2Bx1x^6 - 3Bx1^3x^3 - \frac{1}{2}Bx1^2x^4 + 13Bx1x^5 + \frac{1}{2}Bx1^3x^2 + \frac{19}{4}Bx1^2x^3 \\
& - \frac{63}{4}Bx1x^4 - \frac{9}{4}Bx1^2x^2 + \frac{27}{4}Bx1x^3 + \frac{5}{16}Bx1^2x, 1 \left. \right], \left[ -\frac{3}{4}x + 4x^7 + \frac{25}{16}Bx1x^2 \right. \\
& - \frac{69}{8}x^3 - 2x^6 - \frac{27}{4}x^5 + \frac{1}{16}Bx1 - \frac{1}{2}Bx1x + \frac{57}{16}x^2 + \frac{1}{16} + \frac{23}{2}x^4 + Bx1^4x^7 - 2Bx1^4x^6 \\
& - 8Bx1^3x^7 + 2Bx1^4x^5 + 16Bx1^3x^6 + 20Bx1^2x^7 - Bx1^4x^4 - \frac{33}{2}Bx1^3x^5 - 38Bx1^2x^6 \\
& - 16Bx1x^7 + \frac{1}{4}Bx1^4x^3 + \frac{19}{2}Bx1^3x^4 + \frac{155}{4}Bx1^2x^5 + 24Bx1x^6 - \frac{13}{4}Bx1^3x^3 - \frac{97}{4}Bx1^2x^4 \\
& \left. \left. - 18Bx1x^5 + \frac{1}{2}Bx1^3x^2 + \frac{161}{16}Bx1^2x^3 + \frac{35}{4}Bx1x^4 - \frac{21}{8}Bx1^2x^2 - \frac{27}{8}Bx1x^3 + \frac{5}{16}Bx1^2x, 1 \right] \right]
\end{aligned}$$

```

>
>
>
>
> numer(qq[1][1])

```

$$\begin{aligned}
& 4Bx1^4x^6 - 8Bx1^4x^5 + 8Bx1^4x^4 + 12Bx1^3x^5 - 4Bx1^4x^3 \\
& - 28Bx1^3x^4 + 12Bx1^2x^5 + Bx1^4x^2 + 26Bx1^3x^3 - 5Bx1^2x^4 \\
& - 12Bx1^3x^2 - 16Bx1^2x^3 + 18Bx1x^4 + 2Bx1^3x + 21Bx1^2x^2 \\
& - 27Bx1x^3 + x^4 - 8Bx1^2x + 10Bx1x^2 + Bx1^2 - Bx1x
\end{aligned} \tag{26}$$

> *algcures*[*puiseux*](*numer*(*qq*[1][1]), *x* = 0, *Bx1*, 6)

$$\left\{ \frac{74x^6 + 10x^5 + x^4}{x}, \frac{-170x^6 - 46x^5 - 13x^4 - 2x^3 + x^2}{x}, \frac{-86x^6 - 18x^5 - 3x^4 + 2x^3 + 3x^2 + 2x - 1}{x}, \frac{158x^6 + 38x^5 + 15x^4 + 10x^3 + 10x^2 + 10x - 1}{x} \right\}$$

> # *this looks correct (first puiseux series is a power series with nonnegative coefficients)*

> # *we still have to rule out the other factors*

>

> *algcures*[*puiseux*](*numer*(*qq*[2][1]), *x* = 0, *Bx1*, 6)

$$\left\{ \frac{-1 - 274x^6 - 44x^5 - 7x^4 - x^3 + \frac{5}{2}x}{x}, \frac{-358x^6 - 72x^5 - 17x^4 - 5x^3 - 2x^2 + \frac{1}{2}x}{x}, \frac{278x^6 + 50x^5 + 11x^4 + 2x^3 - 15x^2 - 10x + 1}{x} \right\}$$

> # *nope*

>

> *algcures*[*puiseux*](*numer*(*qq*[3][1]), *x* = 0, *Bx1*, 6)

$$\left\{ \frac{-\frac{1}{2} - 864x^6 - 142x^5 - 24x^4 - 2x^3 + 2x^2}{x}, \frac{-\frac{1}{2} + 608x^6 + 78x^5 + 8x^4 + 2x^3 + 2x^2 + 2x}{x}, \frac{-662x^6 - 100x^5 - 15x^4 - 10x^3 - 10x^2 - 10x + 1}{x} \right\}$$

> # *nope*

>

> *algcures*[*puiseux*](*numer*(*qq*[4][1]), *x* = 0, *Bx1*, 6)

$$\left\{ \frac{-\frac{1}{2} - 1052x^6 - 168x^5 - 28x^4 - 5x^3 - x^2 + \frac{1}{2}x}{x}, \frac{-\frac{1}{2} + 420x^6 + 52x^5 + 4x^4 - x^3 - x^2 + \frac{5}{2}x}{x}, \frac{-458x^6 - 60x^5 - 15x^4 - 10x^3 - 10x^2 - 10x + 1}{x} \right\}$$

> # *nope*

>

>

>

> *Bans* := *numer*(*qq*[1][1])

$$\begin{aligned}
Bans &:= 4Bx1^4x^6 - 8Bx1^4x^5 + 8Bx1^4x^4 + 12Bx1^3x^5 - 4Bx1^4x^3 \\
&- 28Bx1^3x^4 + 12Bx1^2x^5 + Bx1^4x^2 + 26Bx1^3x^3 - 5Bx1^2x^4 \\
&- 12Bx1^3x^2 - 16Bx1^2x^3 + 18Bx1x^4 + 2Bx1^3x + 21Bx1^2x^2 \\
&- 27Bx1x^3 + x^4 - 8Bx1^2x + 10Bx1x^2 + Bx1^2 - Bx1x
\end{aligned} \tag{31}$$

> *Aans* := *Generators*(*EliminationIdeal*(*PI*, {*Ax1*}))[1]

$$Aans := Ax1^2x - Ax1 + 1 \tag{32}$$

> *final\_ans\_factors* := *eliminate*([*Qx1* - (*Ax1* + *Bx1*), *Aans*, *Bans*], [*Ax1*, *Bx1*])[2][1]

$$\begin{aligned}
\text{final\_ans\_factors} := & (4Qx1^4x^8 - 8Qx1^4x^7 + 8Qx1^4x^6 \\
& + 4Qx1^3x^7 - 4Qx1^4x^5 - 12Qx1^3x^6 + 36Qx1^2x^7 + Qx1^4x^4 \\
& + 10Qx1^3x^5 - 71Qx1^2x^6 - 4Qx1^3x^4 + 74Qx1^2x^5 + 18Qx1x^6 \\
& - 42Qx1^2x^4 - 54Qx1x^5 + 49x^6 + 16Qx1^2x^3 + 48Qx1x^4 - 150x^5 \\
& - 2Qx1^2x^2 - 26Qx1x^3 + 188x^4 + 4Qx1x^2 - 126x^3 + 54x^2 \\
& - 12x + 1) (2Qx1^2x^2 - 2Qx1^2x + Qx1^2 + Qx1x - 2Qx1 + x + 1)
\end{aligned} \tag{33}$$

>

> # again, two factors, must decide which

> *poss1* :=  $4Qx1^4x^8 - 8Qx1^4x^7 + 8Qx1^4x^6 + 4Qx1^3x^7 - 4Qx1^4x^5 - 12Qx1^3x^6 + 36Qx1^2x^7 + Qx1^4x^4 + 10Qx1^3x^5 - 71Qx1^2x^6 - 4Qx1^3x^4 + 74Qx1^2x^5 + 18Qx1x^6 - 42Qx1^2x^4 - 54Qx1x^5 + 49x^6 + 16Qx1^2x^3 + 48Qx1x^4 - 150x^5 - 2Qx1^2x^2 - 26Qx1x^3 + 188x^4 + 4Qx1x^2 - 126x^3 + 54x^2 - 12x + 1$

$$\begin{aligned}
\text{poss1} := & 4Qx1^4x^8 - 8Qx1^4x^7 + 8Qx1^4x^6 + 4Qx1^3x^7 \\
& - 4Qx1^4x^5 - 12Qx1^3x^6 + 36Qx1^2x^7 + Qx1^4x^4 + 10Qx1^3x^5 \\
& - 71Qx1^2x^6 - 4Qx1^3x^4 + 74Qx1^2x^5 + 18Qx1x^6 - 42Qx1^2x^4 \\
& - 54Qx1x^5 + 49x^6 + 16Qx1^2x^3 + 48Qx1x^4 - 150x^5 - 2Qx1^2x^2 \\
& - 26Qx1x^3 + 188x^4 + 4Qx1x^2 - 126x^3 + 54x^2 - 12x + 1
\end{aligned} \tag{34}$$

> *algcures*[*puiseux*](*poss1*, *x* = 0, *Qx1*, 6)

$$\left\{ \frac{-212x^6 - 60x^5 - 18x^4 - 4x^3 - x + 1}{x}, \frac{-44x^6 - 4x^5 + 2x^4 + 4x^3 + 4x^2 + 3x - 1}{x}, \frac{32x^6 - 4x^5 - 4x^4 - 2x^3 - x}{x} \right\} \tag{35}$$

> # no

>

> *poss2* :=  $2Qx1^2x^2 - 2Qx1^2x + Qx1^2 + Qx1x - 2Qx1 + x + 1$ :

> *algcures*[*puiseux*](*poss2*, *x* = 0, *Qx1*, 6)

$$\{-128x^5 - 32x^4 - 8x^3 + 2x + 1, 116x^5 + 24x^4 + 6x^3 + 2x^2 + x + 1\} \tag{36}$$

> # yes!

>

> *final\_ans* := *collect*(*subs*(*Qx1* = *F*, *poss2*), *F*, *factor*)

$$\text{final\_ans} := (2x^2 - 2x + 1)F^2 + (x - 2)F + x + 1 \tag{37}$$

> *sols* := *sort*(*simplify*([*solve*(*final\_ans*, *F*)], *symbolic*))

$$\text{sols} := \left[ \frac{-x\sqrt{-8x+1} - x + 2}{4x^2 - 4x + 2}, \frac{x\sqrt{-8x+1} - x + 2}{4x^2 - 4x + 2} \right] \tag{38}$$

> *series*(*sols*[1], *x*, 11)

$$\begin{aligned}
 &1 + x + 2x^2 + 6x^3 + 24x^4 + 116x^5 + 632x^6 + 3720x^7 \\
 &+ 23072x^8 + 148528x^9 + 983072x^{10} + O(x^{11})
 \end{aligned}
 \tag{39}$$

```

>
> # check
> subs(F = -\frac{x - 2 + \sqrt{-8x^3 + x^2}}{2(2x^2 - 2x + 1)}, final_ans)

```

$$\frac{\left(2x^2 - 2x + 1\right)\left(x - 2 + \sqrt{-8x^3 + x^2}\right)^2}{\left(4x^2 - 4x + 2\right)^2} - \frac{\left(x - 2\right)\left(x - 2 + \sqrt{-8x^3 + x^2}\right)}{4x^2 - 4x + 2} + x + 1$$

(40)

```

> simplify(%)

```

0

(41)

```

>
>

```
